# Supplementary material for: ILLUME+: Illuminating Unified MLLM with Dual Visual Tokenization and Diffusion Refinement
Source: arXiv:2504.01934 source file (2025-04-03)
Supplement: Supplementary file 1 [file result_additional_generation.tex]

\begin{table}[ht]
    \centering
    
    \scriptsize
    \vspace{-2mm}
    %\resizebox{\textwidth}{!}{
    \begin{tabular}{lcccccc}
        \toprule
        \textbf{Method} & \textbf{Global} & \textbf{Entity} & \textbf{Attribute} & \textbf{Relation} & \textbf{Other} & \textbf{Overall$\uparrow$} \\
        \midrule
        \multicolumn{7}{c}{\it Generation-specific Models.} \\
        \midrule
        SDv1.5 \cite{rombach2022high} & 74.63 & 74.23 & 75.39 & 73.49 & 67.81 & 63.18 \\
        PixArt-$\alpha$ \cite{chen2023pixart} & 74.97 & 79.32 & 78.60 & 82.57 & 76.96 & 71.11 \\
        Lumina-Next~\cite{liu2024lumina} & 82.82 & 88.65 & 86.44 & 80.53 & 81.82 & 74.63 \\
        SDXL~\cite{podell2023sdxl} & 83.27 & 82.43 & 80.91 & 86.76 & 80.41 & 74.65 \\
        Playground v2.5~\cite{mjhq} & 83.06 & 82.59 & 81.20 & 84.08 & 83.50 & 75.47 \\
        Hunyuan-DiT~\cite{li2024hunyuan} & 84.59 & 80.59 & 88.01 & 74.36 & 86.41 & 78.87 \\
        PixArt-$\Sigma$~\cite{chen2024pixart_sigma} & 86.89 & 82.89 & 88.94 & 86.59 & 87.68 & 80.54\\
        Emu3-Gen~\cite{wang2024emu3} & 85.21 & 86.68 & 86.84 & 90.22 & 83.15 & 80.60 \\
        DALL-E 3~\cite{betker2023improving} & 90.97 & 89.61 & 88.39 & 90.58 & 89.83 & 83.50 \\
        SD3-Medium \cite{stable_diffusion_3} & 87.90 & 91.01 & 88.83 & 80.70 & 88.68 & 84.08 \\
        \midrule
        \multicolumn{7}{c}{\it Unified Understanding and Generation Models} \\
        \midrule
        Janus~\cite{wu2024janus} & 82.33 & 87.38 & 87.70 & 85.46 & 86.41 & 79.68 \\
        Janus-Pro-1B~\cite{chen2025janus_pro} & 87.58 & 88.63 & 88.17 & 88.98 & 88.30 & 82.63 \\
        Janus-Pro-7B~\cite{chen2025janus_pro} & 86.90 & 88.90 & 89.40 & 89.32 & 89.48 & 84.19 \\

        ILLUME~\cite{wang2024illume} & \\
        \textbf{\method-3B} & 84.5 & 83.7 & 85.91 & 89.86 & 86.52 & 79.6 \\
        \bottomrule
    \end{tabular}
    %}
    \caption{Performances on DPG-Bench.}
    \label{tab:exp-dpg}
    \vspace{-4mm}
\end{table}
